# Supplementary material for: Predict and Match: Prophet Inequalities with Uncertain Supply
Source: arXiv:2001.06779 source file (2020-01-22)
Supplement: Supplementary file 1 [file DP-appendix.tex]

\subsection{Super-constant Gap Examples for non-{\em i.i.d.} Buyers}
\label{app:eg}
In the first example, buyer valuations are deterministic and known, and the horizon is MHR. Note that in this setting the order of arrival is also known to the algorithm. The following example shows that no algorithm can be a constant approximation of $\textsc{Pro}$.   
\begin{example}
\label{eg1}
%There is a family of instances when the $h$-th arriving buyer has known value $v_h$, and the horizon distribution $H$ is MHR such that no algorithm can achieve a constant fraction of $\textsc{Pro}$.
%\end{theorem}
%\begin{proof}
Let the horizon distribution be the geometric distribution with parameter $0.5$. Consider a set of $n$ buyers such that  $v_h=2^h$. The expected value of the prophet is $\Theta(n)$ while any algorithm can only achieves a constant value in expectation.
%\end{proof}
\end{example}

In the second example, there are $k$ buyers, and their valuations are deterministic. The arrival is according to a known distribution of permutations. We show that no algorithm can get a constant approximation even if the horizon is a fixed and known to be $n \leq k$. 
\begin{example}
\label{eg2}
Let $k=2(n-1)+1$ and $v_j= 2^{j+1}$ if $j < n$ and $v_j=0$ otherwise. The arrival order of buyers is one of the following $k+1$ permutations: For $1 \le i \le n-1$, permutation $\pi_i = \left(1,2, \dots i, n, n+1, \ldots, k, i+1, \ldots, n-1 \right)$ is chosen with probability $\frac{1}{2^i}$ and permutation $\pi_{n}= \left(n, n+1, \ldots, k, 1,2,\ldots n-1 \right)$ is chosen with probability $\frac{1}{2^{n-1}}$. 

Any policy can only generate O(1) in expectation while the value of the prophet is $\Theta(n)$. Note that this is tight because randomly picking one of the first $n$ buyers is a $\Theta(n)$-approximation.  
\end{example}

\subsection{Proof of Lemma~\ref{lem:VPRO-LP}}
\label{app:VPRO-LP}
We defined variable $y_{ivh}$ as the probability that $h$-th buyer has value $v$ and is assigned to item $i$, given that item $i$ has not departed before $h$ (its horizon is not less than $h$). The first set of constraints simply state that a specific type of buyer only can be chosen when it appears. For the second set of constraints, note that the prophet at step $h$ can only know if the horizon of an item is less than $h$ or not. Let's assume the only difference between two instances of the problem is the realization of the horizon of the $i$-th item: in the first instance it is $h$ and in the second instance it is $h' > h$. The first $h$ decision of the prophet would be the same for these two instances because those are exactly the same from the prophet view until time $h$. In addition, for any realization of the horizon of the $i$-th item it can only be chosen once. Therefore, we only write the constraint when the horizon distribution is $n$ which is the strongest constraint.

\subsection{Proof of Theorem~\ref{thm:DPConst}}
\label{app:DPConst}
Consider any tuple $(i,v,h)$. The expected value of this tuple in the LP optimal solution ($\textsc{Opt}$) is $y_{ivh} \Pr[Z_i \ge h] \cdot v$. Now, we compute the expected value from this tuple in the $\textsc{Alg}$ denoted by $A_{ivh}$:

$\textsc{Alg}$ only get the value $v$ from this tuple if the $h$-th buyer announces value $v$ and item $i$ be the first item in the arbitrary order of item satisfying the three conditions mentioned in the algorithm. 
\begin{align*}
A_{ivh} \ge & \frac{y_{ivh}}{2} \cdot \Pr[Z_i \ge h] \cdot v \cdot \Pr[\text{no other buyer assigned to item $i$}] \cdot\\
&\Pr[\text{no other item  assigned to buyer $h$}].
\end{align*}

Using the second set of constraints, the expected number of buyers assigned to an item $i$ is at most $0.5$: 
$$\E[\#\text{buyers assigned to $i$}] \le \sum_{v,h} \frac{y_{ivh}}{2 \Pr[X_h=v]} \cdot \Pr[X_h=v] \le \frac{1}{2}.$$
Therefore, using Markov's inequality we have:
$$\Pr[\text{no other buyer assigned to $i$}] \ge \frac{1}{2}.$$

Similarly, using the first set of constraints we have:
$$\E[\# \text{ items assigned to $h$-th buyer announcing value $v$}] \le \sum_{i} \frac{y_{ivh}}{2 \Pr[X_h=v]} \cdot \Pr[Z_i \ge h] \le \frac{1}{2}.$$
Therefore, using Markov's inequality we have:
$$\Pr[\text{no other item assigned to $h$-th buyer}] \ge \frac{1}{2}.$$
Now, we have:
$$A_{ivh} \ge \frac{y_{ivh}}{8}  \Pr[Z_i \ge h] \cdot v,$$
which is $\frac{1}{8}$-fraction of the expected value of this tuple in the $\textsc{Opt}$. Using linearity of expectation completes the proof.

\section{Pricing Scheme Implementation of the Algorithm in Section~\ref{sec:DPConst}}
\label{app:pricingScheme}

In Section~\ref{sec:DPConst}, we found an upper bound for $\textsc{VPro}$ by an LP. In other words, prophet behavior and any other possible policy without information about horizons realization including the optimal algorithm ($\textsc{Alg*}$) is a feasible solution for the presented LP. Now we strengthen that LP by adding the following set of constraints: 
\begin{equation}
\label{eq:newConst}
\frac{y_{iv_1h}}{\Pr[X_h=v_1]}  \le \frac{y_{iv_2h}}{\Pr[X_h=v_2]},\quad \forall h,i, v_1 \le v_2.
\end{equation}
It is easy to see that $\textsc{VPro}$ does not satisfy the new constraints necessarily. However, we claim that $\textsc{Alg*}$ which is the optimal algorithm knowing only the value and horizon distributions satisfies them.

\begin{lemma}
	\label{lem:newLPAlg*}
	Let $y_{ivh}$ be the probability that $\textsc{Alg*}$ assigns the $h$-th buyer to item $i$ and the value of that buyer is $v$, given that item $i$ has not departed (its horizon is not less than $h$). For any fixed $i$ and $h$, $\frac{y_{ivh}}{\Pr[X_h=v]}$ is non-decreasing in $v$.  
\end{lemma}
\begin{proof}
For any $v_1 < v_2$, consider two instance such that the information of the optimal policy at time $h$ is the same for the two instances except that in the first one $X_h = v_1$ and in the second one $X_h=v_2$. Given that in the first instance $X_h = v_1$ and $X_h=v_2$ in the second instance, the probability of occurring any same set of information (including the other values before time $h$ and departures before this time) is equal for the two instances.

Consider one specific realization in which set $S$ of items has not departed at step $h$ (departures before time $h$ happen exactly the same way for both instances). The main claim is as follows: assuming that optimal policy always uses the same tie breaking procedure if it assigns an item $i$ to $h$-th buyer in the first instance, it does the same in the second instance. This is because before time $h$ both instances are exactly the same and all the assignments are the same (the argument works in the presence of randomized decisions too). Let $S' \subseteq S$ be the set of items has not departed or assigned to a buyer before $h$.  Let $\textsc{Alg*}(S,h+1)$ shows the expected value of the optimal policy after time $h$ given the information so far (the policy does not have the information about departure at time $h$ yet).  At time $h$, the policy assigns an available item $i\in S' $ to buyer $h$ only if $\textsc{Alg*}(S' \setminus\{i\} , h+1) \le \textsc{Alg*}(S' \setminus\{i'\})$ for any $i' \in S'$ and $v_1 + \textsc{Alg*}(S' \setminus\{i\} , h+1) > \textsc{Alg*}(S',h+1)$. It is obvious that if $v_1$ satisfies the two constraints for item $i$, then $v_2$ satisfies them too for the same $i$.

Now, we have seen that given that $X_h =v_2$ the probability of assigning any item to the $h$-th buyer is greater than the same probability given that $X_h =v_1$ for the same instances. Taking the expectation over all the possibilities completes the proof.    
\end{proof}
\begin{lemma}
	Let $\textsc{Opt}$ be the optimal solution of the new LP (with the newly added set of Constraints $\left(\ref{eq:newConst}\right)$ : 
	$$8 \textsc{Opt} \ge \textsc{VPro}.$$
\end{lemma} 
\begin{proof}
In Theorem~\ref{thm:DPConst} we show that there is an algorithm such that: $ 8 \textsc{Alg} \ge \textsc{VPro}$. Therefore, it suffices to show that $\textsc{Opt} \ge \textsc{Alg}$. Let $\textsc{Alg*}$ denote the optimal policy. From Lemma~\ref{lem:newLPAlg*} we know that $Alg*$ corresponds to a feasible solution of this LP and therefore $\textsc{Opt} \ge \textsc{Alg*} \ge \textsc{Alg}$ completing the proof. 
\end{proof} 

Now we modify the algorithm in Section~\ref{sec:DPConst} and present a pricing scheme which is truthful. Let $v_1 < v_2, \dots <v_k$ be the possible values of $h$-th buyer. Instead of asking the arriving buyer at time $h$ their value, we do the following:

\begin{algorithm}[htbp]
\DontPrintSemicolon
\KwData{$h$}
\Begin{
\For{$j=1, ... , k$}
{
$S_j \gets \varnothing$\;
\For{item $i$}{
\If{$\forall z < j: i \notin S_z$}{
with probability $\frac{y_{i,v_j,h}}{2\Pr[X_h=v_j]} - \frac{y_{i,v_{j-1},h}}{2\Pr[X_h=v_{j-1}]}$ place item $i$ in $S_j$

\tcc*{with probability $\frac{y_{i,v_1,h}}{2\Pr[X_h=v_1]}$ for $j=1$}
}
}
}
Find the smallest $j$ such that: $S_j$ contains an available item (has not departed or assigned)\;
Set the price $p= v_j$ and choose that available item in $S_j$ as the potential match \;
\If{$h$-th buyer accepts the price $p$} {
Assign the possible match to the $h$-th buyer and charge price $p$
 
\tcc*{If no possible match has been found, $p = \infty$}
}
}
\caption{Pricing Scheme Competing with $\textsc{VPRo}$}\label{alg:Alg2}
\end{algorithm}

\begin{theorem}
Let $\textsc{Alg}'$ be the expected welfare of the Algorithm~\ref{alg:Alg2}: 
	 $$8 \textsc{Alg}' \ge \textsc{Opt} \ge \frac{1}{8} \textsc{VPro}.$$    
\end{theorem}
\begin{proof}
If the actual value of the $h$-th buyer is $v_j$, she accepts any price which is not more than $v_j$. Consider the set $S =\bigcup_{t=1} ^j S_t$. We can see that each item $i$ is in $S$ with probability $\frac{y_{iv_jh}}{2 \Pr[X_h=v_j]}$. Now, if we consider an order of items such that items in $S_t$ appear before $S_{t'}$ if $t < t'$, then we can see that Algorithm~\ref{alg:Alg2} and the algorithm in Section~\ref{sec:DPConst} are the same, and the same analysis shows that this algorithm is an $8$-approximation of the optimal solution of the new LP which completes the proof.
\end{proof}
